# Supplementary material for: Evaluation of Model-Based PM$_{2.5}$ Estimates for Exposure Assessment During Wildfire Smoke Episodes in the Western U.S
Source: arXiv:2209.01479 source file (2023-01-09)
Supplement: Supplementary file 1 [file Supporting_Info.tex]

% \documentclass[journal=esthag,manuscript=article]{achemso}
% \usepackage{amsmath}
% \usepackage{graphicx}
% \usepackage{subcaption}
% \usepackage{float}

% \usepackage{etoolbox} % needed for patch
% \makeatletter
% \patchcmd{\acs@contact@details}{E}{*\,E}{}{}
% \patchcmd{\acs@email@list@aux}{;}{\par*\,Email}{}{}
% \makeatother

% \renewcommand{\thepage}{S\arabic{page}}

% \renewcommand{\thefigure}{S\arabic{figure}}
% \renewcommand{\thetable}{S\arabic{table}}

% \title{Supporting Information for "Evaluation of Model-Based PM$_{2.5}$ Estimates for Exposure Assessment During Wildfire Smoke Episodes in the Western U.S."}

% \author{Ellen M. Considine}
% \email{ellen_considine@g.harvard.edu}
% \author{Jiayuan Hao}
% \affiliation{Department of Biostatistics, Harvard T.H. Chan School of Public Health, Boston, Massachusetts, 02115, USA.}
% \author{Priyanka deSouza}
% \affiliation{Department of Urban and Regional Planning, University of Colorado Denver, University of Colorado Denver, Denver, Colorado, 80202, USA.}
% \alsoaffiliation{CU Population Center, University of Colorado Boulder, Boulder, Colorado, 80309, USA.}
% \author{Danielle Braun}
% \affiliation{Department of Biostatistics, Harvard T.H. Chan School of Public Health, Boston, Massachusetts, 02115, USA.}
% \alsoaffiliation{Department of Data Science, Dana-Farber Cancer Institute, Boston, Massachusetts, 02215, USA.}
% \author{Colleen E. Reid}
% \affiliation{Department of Geography, University of Colorado Boulder, Boulder, Colorado, 80302, USA.}
% \alsoaffiliation{CU Population Center, University of Colorado Boulder, Boulder, Colorado, 80309, USA.}
% \alsoaffiliation{Earth Lab, University of Colorado Boulder, Boulder, Colorado, 80303, USA.}
% \author{Rachel C. Nethery}
% \affiliation{Department of Biostatistics, Harvard T.H. Chan School of Public Health, Boston, Massachusetts, 02115, USA.}

% \begin{document}

% \maketitle

% \textbf{Contents:} 14 pages; equations, supplemental notes, 2 figures, and 8 tables

% \pagebreak

% \section{Comparison Metrics Equations}
% % METRICS EQUATIONS:

% \begin{equation}
%     \text{Mean Bias}(\textbf{x},\textbf{y}) = \frac{1}{n}\sum_{i=1}^n(y_i-x_i)
% \end{equation}

% \begin{equation}
%     \text{Normalized Mean Bias}(\textbf{x},\textbf{y}) = \frac{\sum_{i=1}^n(y_i-x_i)}{\sum_{i=1}^n x_i}
% \end{equation}

% \begin{equation}
%     \text{Median Absolute Difference}(\textbf{x},\textbf{y}) = Median\Big\{|y_i-x_i|\Big\}_{i=1}^n
% \end{equation}

% \begin{equation}
%     \text{Median Ratio}(\textbf{x},\textbf{y}) = Median\Big\{y_i/x_i\Big\}_{i=1}^n
% \end{equation}

% \begin{equation}
%     \text{Mean Ratio}(\textbf{x},\textbf{y}) = \frac{1}{n}\sum_{i=1}^n(y_i/x_i)I(x_i > 0)
% \end{equation}

% \begin{equation}
%     \text{Root-Mean Squared Difference}(\textbf{x},\textbf{y}) = \sqrt{\frac{1}{n}\sum_{i=1}^n(y_i-x_i)^2}
% \end{equation}

% \begin{equation}
%     R^2(\textbf{x},\textbf{y}) = \Bigg[\frac{\sum_{i=1}^n(y_i-\bar{y})(x_i - \bar{x})}{\sqrt{\sum_{i=1}^n(y_i-\bar{y})^2\sum_{i=1}^n(x_i-\bar{x})^2}} \Bigg]^2
% \end{equation}

% For spatial RMSD and $R^2$, replace individual observations with location-averages (across all the days). For temporal RMSD and $R^2$, replace individual observations with daily averages (across all locations).

% \pagebreak

% \section{Supplemental Notes}

% \subsection{Investigating Large Mean Ratios}

% In the Results, we noted that the mean ratio between the Reid estimates and the smoke monitor observations was affected by 18 instances where the monitor observations were in their lowest quartile ($ < 4\mu g/m^3$) and the model estimates were high ($ > 35.5 \mu g/m^3$). Of these, four of the Reid estimates were over 55.5$\mu g/m^3$; the maximum was 68.6$\mu g/m^3$. Among these 18 instances, all but one were in the warm season (and the one was in April). A large cluster of the over-predictions were in northern California in 2015, at a location bordered by half a dozen large fires in its bordering counties. 

% \subsection{Results of the AQI Classification Analysis}

% The AQI classifications analysis was motivated by the possibility of health scientists using a categorical exposure instead of a continuous one (perhaps in an attempt to address the issue of large prediction errors at high concentrations of PM$_{2.5}$). Table S3 gives the frequencies with which the Di and Reid models predicted each AQI class compared with the observations from the smoke monitors. The marginal frequencies illustrate that the Reid model better captures the empirical AQI class distribution than the Di model. However, neither model correctly classified any of the 58 smoke monitor observations in the highest AQI category ("Hazardous", defined as $\geq 250.5 \mu g/m^3$).

% Table S4 reports that the Reid dataset has both a lower total AQI misclassification rate than the Di dataset (20.7\% vs 23.2\% respectively) and a lower rate of large misclassifications (misclassification by more than one level of the AQI; 2.2\% and 2.6\% for Reid and Di respectively), which may cause more issues for health analyses than single-level misclassifications. Looking into the direction of misclassification for each dataset (also in Table S4): Di has a higher under-classification rate (15.8\% compared with Reid's 11.0\%), but Reid has a higher over-classification rate (9.7\% compared with Di's 7.5\%). It is unclear whether these two cases (over- and under-classification) might differentially bias health effect estimates based on a categorical PM$_{2.5}$ exposure.  

% \subsection{Results of the Binary Smoke / Nonsmoke Classification Analysis}

% Tables S5 and S6 explore what would happen if, instead of all the AQI classes, we considered a binary classification of "non-smoke" (PM$_{2.5} < 35.5 \mu g/m^3$ -- grouping "Good" and "Moderate"; n = 18,816) and "smoke" (PM$_{2.5} \geq  35.5\mu g/m^3$ -- grouping "Unhealthy for Sensitive Groups" and above; n = 1,034), which is a concept used in many epidemiological studies of wildfire smoke exposure.$^{34, 7}$ % \cite{liu_2017, reid_2016}. 
% Here, we see that the overall misclassification rates for the Di and Reid models are exactly the same (3.4\%). Considering "smoke" to be the exposure of interest, the two models' specificities and negative predictive values are also quite similar (all $>$ 95\%). However, the Reid model has a substantially higher sensitivity (28.2\% compared to Di's 10.5\%) and the Di model has a higher positive predictive value (67.5\% compared to Reid's 55.2\%). 

% \subsection{Results of the Sensitivity Analysis Unweighted By Population Density}

% The main comparison metrics unweighted by population density are given in Table S2. This sensitivity analysis shows that while the magnitudes of the metrics are affected by population density weighting (some getting better and some getting worse), our conclusions were unchanged (i.e., the metrics getting worse for higher levels of PM$_{2.5}$ and the Reid estimates performing better than the Di estimates). One other note is that in the results unweighted by population density, both the spatial and temporal correlations (for both the Di and Reid estimates) for high PM$_{2.5}$ were negative, rather than in our main analysis this was only true for the temporal correlations.

% Tables S4 and S6 provide results of the categorical analyses (all AQI levels and binary smoke/non-smoke respectively) unweighted by population density (in addition to those weighted by population density). Again, although the magnitudes of these metrics are affected by population density-weighting, the main conclusions do not change, with the exception of the Di estimates having slightly less total misclassifications than the Reid estimates (the opposite of what the weighted analysis shows). 


% \subsection{Results of the Sensitivity Analysis on the Reid Estimates without CMAQ (Including 2017-2018)}

% Table S7 provides the comparison metrics for the Reid estimates and smoke monitor observations in 2017-2018 (beyond the temporal coverage of the Di estimates). These metrics similarly display worse performance at higher levels of PM$_{2.5}$, but in general are better than the 2008-2016 metrics, especially for higher levels of PM$_{2.5}$. For instance, the 2017-2018 RMSD and $R^2$ for high PM$_{2.5}$ were 54.6$\mu g/m^3$ and 0.45, whereas for 2008-2016 they were 142.4$\mu g/m^3$ and 0.01 respectively. It is unlikely that this improved performance is attributable to omission of the CMAQ variable from the model (as opposed to the model trained with CMAQ, which is unavailable for 2017-2018), as the comparison metrics from 2008-2016 across the with/without CMAQ models are very similar (e.g., the 2008-2016 high PM$_{2.5}$ Reid without CMAQ RMSD was 144.1$\mu g/m^3$ and $R^2$ was 0.01, shown in Table S7). Instead, we infer that more smoke monitors being deployed in these later years increased the availability of smoke-specific data used to train the Reid model.

% \subsection{Results of the Sensitivity Analysis Comparing Reid and Di to EPA Monitor Observations}

% Looking more broadly than wildfire smoke, Table S8 provides the comparison metrics for the Di and Reid estimates compared to EPA monitor observations (2008-2016). Unsurprisingly, given that EPA monitor observations were part of both models' training data and tend to have less extreme values of PM$_{2.5}$ than the smoke monitor data, both the Di and Reid estimates exhibit better accuracy with respect to the EPA monitor observations than to the smoke monitor validation set. For instance, the RMSD and $R^2$ for overall PM$_{2.5}$ in the main analysis were 29.3$\mu g/m^3$ and 0.07 for Di and 27.8$\mu g/m^3$ and 0.15 for Reid, whereas compared to the EPA monitors they were 3.9$\mu g/m^3$ and 0.72 for Di and 2.8$\mu g/m^3$ and 0.85 for Reid. This improved performance could simply be due to the models over-fitting to their training data.

% The spatial and temporal versions of RMSD and correlation (in addition to the regular versions, given in the previous paragraph) illustrate that the Reid estimates describe major variability in the EPA monitor data better than the Di estimates, across levels of PM$_{2.5}$ (Table S8). This is likely due to the Reid model focusing on the western US instead of the whole country -- PM$_{2.5}$ variability in the east may look quite different than in the west, the latter being very affected by wildfire smoke variability. By contrast, the bias and ratio metrics are more mixed across levels of PM$_{2.5}$, with some showing Reid as better compared to the EPA monitor data and others showing Di as better (Table S8). For instance, for high PM$_{2.5}$, the mean bias for Di is better than for Reid (-5.7 vs -7.8$\mu g/m^3$ respectively) but the median absolute difference for Di is worse than for Reid (7.8 vs 6.9$\mu g/m^3$ respectively). This mixed finding could be due to the Di estimates' finer spatial resolution, which facilitates estimation of more localized air pollution hotspots (e.g. urban or industrial sources, rather than wildfire smoke).
 
% \pagebreak

% \section{Supplemental Figures and Tables}
% % \subsection{No Missingness}

% \begin{figure}[!hb]
% \begin{centering}
% \includegraphics[width=1\linewidth]{figures/Seasonal_differences.pdf} 
%   \caption{Maps of the seasonal differences (Reid - Di) between county-level averages (2008-2016) of the model-based estimates. We define Spring as March-May, Summer as June-August, Autumn as September-November, and Winter as December-February.}
%   \label{fig:seasonal}
% \end{centering}
% \end{figure}

% \begin{figure}[!hb]
% \begin{centering}
% \includegraphics[width=0.85\linewidth]{figures/Validation_Monitor_Obs.pdf} 
%   \caption{Map of all smoke monitor observations in the validation set, colored by the number of days they were deployed.}
%   \label{fig:monitors}
% \end{centering}
% \end{figure}

% \begin{table}[!hb]
% \centering
% \begin{tabular}{|p{3.2cm} | p{1.2cm} p{0.9cm} p{0.9cm} | p{1.2cm} p{0.9cm} p{0.9cm}| p{1.2cm} p{0.9cm} p{1.2cm} |}
%   \hline
%   & \multicolumn{3}{c|}{\textbf{Overall (N = 19,850)}}  & \multicolumn{3}{c|}{\textbf{Medium (N = 5,432)}} & \multicolumn{3}{c|}{\textbf{High (N = 1,034)}} \\
%   \hline
% \textbf{Subset \mbox{(N$_O$, N$_M$, N$_H$)}} & Monitor & Di & Reid & Monitor & Di & Reid & Monitor & Di & Reid \\ 
%   \hline
% %   \multicolumn{10}{|c|}{\textbf{Season}} \\
%   Arizona \mbox{(159, 6, 0)} & 6.07 (3.24) & 6.31 (2.5) & 5.58 (2.95) & 19.96 (6.13) & 7.05 (1.08) & 7.63 (3.26) & NA (NA) & NA (NA) & NA (NA) \\ 
%   \hline
% California \mbox{(14550, 4526, 729)} & 11.5 (14.86) & 7.73 (5.6) & 10.46 (6.45) & 22.73 (23.89) & 11.66 (7.33) & 15.11 (9.03) & 74.25 (69.62) & 16.96 (16.49) & 23.56 (21.86) \\ 
%   \hline
% Colorado \mbox{(379, 42, 31)} & 7.52 (10.33) & 5.54 (2.48) & 5.78 (2.71) & 30.61 (74.52) & 5.19 (1.86) & 4.55 (6.24) & 110.51 (175.69) & 5.8 (3.29) & 11.14 (14.17) \\ 
%   \hline
% Idaho \mbox{(1983, 461, 138)} & 10 (14.5) & 10.79 (8.72) & 12.7 (11.31) & 24.87 (24.73) & 17.34 (12.83) & 23.71 (16.93) & 58.66 (46.12) & 32.08 (18.36) & 43.09 (17.6) \\ 
%   \hline
% Montana \mbox{(614, 99, 30)} & 7.93 (18.43) & 10.21 (11.63) & 7.83 (10.97) & 33.91 (35.41) & 24.72 (21.97) & 24.79 (17.98) & 73.22 (51.22) & 47.79 (31.3) & 41.18 (21.48) \\ 
%   \hline
% \mbox{New Mexico} \mbox{(938, 85, 45)} & 10.24 (44.18) & 4.77 (3.64) & 9.43 (8.5) & 79.84 (135.08) & 6.9 (5.63) & 18.8 (12.26) & 168.31 (194.63) & 2.75 (2.24) & 14.83 (9.91) \\ 
%   \hline
% Oregon \mbox{(262, 66, 35)} & 19.32 (73.6) & 6.42 (4.43) & 11.73 (11.47) & 74.78 (141.26) & 9.46 (6.13) & 27.15 (11.55) & 99.51 (165.65) & 8.46 (5.51) & 30.72 (11.4) \\ 
%   \hline
% Utah \mbox{(12, 1, 1)} & 9.3 (31.96) & 2.2 (0.55) & 8.75 (4.1) & 129.04 (NA) & 3.25 (NA) & 5.1 (NA) & 129.04 (NA) & 3.25 (NA) & 5.1 (NA) \\ 
%   \hline
% Washington \mbox{(906, 140, 22)} & 26.82 (84.14) & 11.21 (12.57) & 16.92 (38.44) & 104.89 (162.55) & 27.17 (19.5) & 56.35 (71.56) & 273.23 (200.32) & 50.61 (15.98) & 141.83 (64.64) \\ 
%   \hline
% Wyoming \mbox{(47, 6, 3)} & 1.65 (1.42) & 3.5 (1.58) & 2.9 (0.93) & 33.86 (8.25) & 20.6 (11.15) & 26.08 (8.65) & 40.35 (3.13) & 28.9 (8.04) & 26.41 (3.05) \\ 
%   \hline
% \end{tabular}
% \caption{\label{tab: main-states} Mean (standard deviation) weighted by population density for each data source and level of PM$_{2.5}$ in the validation set, by state. All values are in $\mu g/m^3$. As described in the main text, "Overall" refers to the entire validation dataset; "Medium" refers to PM$_{2.5} \geq 12.1\mu g/m^3$ as measured by the smoke monitors, corresponding to Yellow AQI and above; "High" refers to PM$_{2.5} \geq 35.5\mu g/m^3$ as measured by the smoke monitors, corresponding to Orange AQI and above. }
% \end{table}

% \begin{table}[!h]
% \centering
% \begin{tabular}{|p{3.6cm} | p{1.5cm} p{1.5cm} |  p{1.5cm} p{1.5cm} | p{1.5cm} p{1.5cm}|}
%   \hline
%   & \multicolumn{2}{p{3cm}|}{\textbf{Overall \mbox{(N = 19,850)}}}  & \multicolumn{2}{p{3cm}|}{\textbf{Medium \mbox{(N = 5,432)}}} & \multicolumn{2}{p{3cm}|}{\textbf{High \mbox{(N = 1,034)}}} \\
%   \hline
% \textbf{Metric \mbox{(Optimal} Value)} & Di vs. \mbox{Monitor} & Reid vs. \mbox{Monitor} & Di vs. \mbox{Monitor} & Reid vs. \mbox{Monitor} & Di vs. \mbox{Monitor} & Reid vs. \mbox{Monitor} \\ 
%   \hline
%   Mean Bias (0) & -6.10 & -2.16 & -20.87 & -12.40 & -73.60 & -52.66 \\ 
%   \hline
% Normalized \mbox{Mean Bias (0)} & -0.46 & -0.16 & -0.63 & -0.37 & -0.77 & -0.55 \\ 
%   \hline
% \mbox{Median Absolute} \mbox{Difference} (0) & 3.08 & 3.07 & 10.92 & 9.17 & 42.78 & 33.52 \\ 
%   \hline
% \mbox{Median Ratio (1)} & 0.74 & 1.03 & 0.42 & 0.61 & 0.22 & 0.49 \\ 
%   \hline
%  Mean Ratio (1) & 1.67 & 2.49 & 0.52 & 0.81 & 0.33 & 0.63 \\ 
%   \hline
% RMSD (0) & 32.42 & 31.13 & 61.66 & 58.65 & 139.06 & 130.69 \\ 
%   \hline
% $R^2$ (1) & 0.13 & 0.16 & 0.07 & 0.10 & 0.02 & 0.02 \\ 
%   \hline
% \mbox{Spatial RMSD (0)} & 66.59 & 64.97 & 111.12 & 108.57 & 158.56 & 153.32 \\ 
%   \hline
% \mbox{Temporal RMSD (0)} & 12.32 & 11.57 & 64.77 & 63.59 & 151.11 & 145.62 \\ 
%   \hline
% Spatial \mbox{Correlation (1)} & 0.20 & 0.24 & -0.03 & 0.03 & -0.16 & -0.11 \\ 
%   \hline
% Temporal \mbox{Correlation (1)} & 0.38 & 0.41 & 0.05 & 0.08 & -0.08 & -0.05 \\ 
%   \hline
% \end{tabular}
% \caption{\label{tab: UNW-metrics} Metrics \textit{unweighted by population density} comparing the Di estimates and Reid estimates to the smoke monitor observations (2008-2016), stratified by PM$_{2.5}$ level. Counterpart to Table 2 in the main text. All metrics except for median ratio, mean ratio, $R^2$, and spatial/temporal correlation are in $\mu g/m^3$.}
% \end{table}

% \begin{table}[!hb]
% \centering
% \begin{subtable}[c]{\textwidth}
% \begin{tabular}{|r|rrrrrr|r|}
%     \hline
%  & \multicolumn{6}{|c|}{Di AQI Class} \\
%   \hline
% Monitor AQI Class & 1 & 2 & 3 & 4 & 5 & 6 & Marginals \\ 
%   \hline
% 1 & 13801 & 609 & 6 & 2 & 0 & 0 & 14418 \\ 
%   2 & 3289 & 1040 & 47 & 22 & 0 & 0 & 4398 \\ 
%   3 & 219 & 209 & 24 & 25 & 0 & 0 & 477 \\ 
%   4 & 168 & 174 & 51 & 20 & 3 & 0 & 416 \\ 
%   5 & 29 & 27 & 9 & 17 & 1 & 0 & 83 \\ 
%   6 & 31 & 9 & 3 & 13 & 2 & 0 & 58 \\ 
%   \hline
%   Marginals & 17537 & 2068 & 140 & 99 & 6 & 0 & 19850 \\ 
%   \hline
%   Percent Change (\%) & +22 & -53 & -71 & -76 & -93 & -100 \\
%   \hline
% \end{tabular}
% \caption{Di classifications compared to smoke monitor classifications}
% \vspace{5mm}
% \end{subtable}
% \begin{subtable}[c]{\textwidth}
% \begin{tabular}{|r|rrrrrr|r|}
%     \hline
%  & \multicolumn{6}{|c|}{Reid AQI Class} \\
%   \hline
% Monitor AQI Class & 1 & 2 & 3 & 4 & 5 & 6 & Marginals \\ 
%   \hline
% 1 & 12976 & 1321 & 85 & 36 & 0 & 0 & 14418 \\ 
%   2 & 2713 & 1327 & 211 & 145 & 2 & 0 & 4398 \\ 
%   3 & 115 & 193 & 78 & 89 & 2 & 0 & 477 \\ 
%   4 & 72 & 126 & 87 & 127 & 4 & 0 & 416 \\ 
%   5 & 16 & 6 & 9 & 43 & 9 & 0 & 83 \\ 
%   6 & 23 & 5 & 3 & 22 & 5 & 0 & 58 \\
%   \hline
%   Marginals & 15915 & 2978 & 473 & 462 & 22 & 0 & 19850 \\
%   \hline
%   Percent Change (\%) & +10 & -32 &  -1 &  +11 & -73 & -100   \\
%   \hline
% \end{tabular}
% \caption{Reid classifications compared to smoke monitor classifications}
% \end{subtable}
% \caption{\label{tab: AQI classes} Frequency tables for the Di and Reid estimates' classification of the AQI in the validation set. Levels 1-6 of the AQI are described in Methods: Analysis.}
% \end{table}

% \begin{table}[!hb]
% \centering
% \begin{tabular}{|p{3cm}|r|r|r|r|r|r|}
%   \hline
%  \textbf{Comparison} & \textbf{Misclassified} & \textbf{Underclassified} & \textbf{Overclassified} & \textbf{Large Misclass.} \\ 
%   \hline
% \mbox{Di vs Monitor}, weighted & 23.22 & 15.75 & 7.47 & 2.58 \\ 
%   \hline
% \mbox{Reid vs Monitor}, weighted & 20.69 & 11.02 & 9.67 & 2.17 \\ 
%   \hline
% \mbox{Di vs Monitor}, unweighted & 25.01 & 21.41 & 3.60 & 3.59 \\ 
%   \hline
% \mbox{Reid vs Monitor}, unweighted & 26.87 & 17.32 & 9.55 & 3.36 \\ 
%   \hline
% \end{tabular}
% \caption{\label{tab: main-AQI} AQI classification metrics for the Di and Reid estimates compared with the smoke monitor observations, weighted and unweighted by population density.}
% \end{table}


% \begin{table}[!hb]
% \centering
% \begin{subtable}[c]{\textwidth}
% \begin{tabular}{|r|rr|r|}
%     \hline
%  & \multicolumn{2}{|c|}{Di Binary Exposure} \\
%   \hline
% Monitor Binary Exposure & Non-smoke & Smoke & Marginals \\
%   \hline
% Non-smoke & 18739 & 77 & 18816 \\ 
%   Smoke & 866 & 168 & 1034 \\ 
%   \hline
%   Marginals & 19605 & 245 & 19850 \\
%   \hline
% \end{tabular}
% \caption{Di classifications compared to smoke monitor classifications}
% \vspace{5mm}
% \end{subtable}
% \begin{subtable}[c]{\textwidth}
% \begin{tabular}{|r|rr|r|}
%     \hline
%  & \multicolumn{2}{|c|}{Reid Binary Exposure} \\
%   \hline
% Monitor Binary Exposure & Non-smoke & Smoke & Marginals \\
%   \hline
% Non-smoke & 18337 & 479 & 18816 \\ 
%   Smoke & 556 & 478 & 1034 \\
%   \hline
%   Marginals & 18893 & 957 & 19850 \\  
%   \hline
% \end{tabular}
% \caption{Reid classifications compared to smoke monitor classifications}
% \end{subtable}
% \caption{\label{tab: binary classes} Frequency tables for the Di and Reid estimates' binary classification of AQI as Non-smoke ("Good" or "Moderate") vs. Smoke ("Unhealthy for Sensitive Groups" and above) in the validation set.}
% \end{table}

% \begin{table}[!hb]
% \centering
% \begin{tabular}{|p{3cm}|r|r|r|r|r|r|}
%   \hline
%  \textbf{Comparison} & \textbf{Misclassified} & \textbf{Sensitivity} & \textbf{Specificity} & \textbf{PPV} & \textbf{NPV} \\ 
%   \hline
% \mbox{Di vs Monitor}, weighted & 3.44 & 10.51 & 99.81 & 67.50 & 96.73 \\ 
%   \hline
% \mbox{Reid vs Monitor}, weighted & 3.44 & 28.24 & 99.13 & 55.19 & 97.34 \\ 
%   \hline
% \mbox{Di vs Monitor}, unweighted & 4.75 & 16.25 & 99.59 & 68.57 & 95.58 \\ 
%   \hline
% \mbox{Reid vs Monitor}, unweighted & 5.21 & 46.23 & 97.45 & 49.95 & 97.06 \\ 
%   \hline
% \end{tabular}
% \caption{\label{tab: binary-summary} Summary statistics for the Di and Reid estimates' binary classification of AQI as Non-smoke ("Good" or "Moderate") vs. Smoke ("Unhealthy for Sensitive Groups" and above) in the smoke monitor validation set, weighted and unweighted by population density. PPV = positive predictive value, NPV = negative predictive value.}
% \end{table}

% % \section{Tables for Sensitivity Analysis}

% % \begin{table}[!hb]
% % \centering
% % \begin{tabular}{|p{2cm} | ccc | ccc | ccc |}
% %   \hline
% %   & \multicolumn{3}{c|}{\textbf{Overall (N = 29,109)}}  & \multicolumn{3}{c|}{\textbf{Medium (N = 7,868)}} & \multicolumn{3}{c|}{\textbf{High (N = 1,737)}} \\
% %   \hline
% % \textbf{Metric} & Monitor & Di & Reid & Monitor & Di & Reid & Monitor & Di & Reid \\ 
% %   \hline
% %     Minimum & 0.00 & 0.00 & 0.00 & 12.12 & 0.00 & 0.14 & 35.50 & 0.00 & 0.63 \\ \hline
% %   1st \mbox{Quartile} & 4.04 & 3.32 & 4.80 & 14.50 & 5.75 & 8.10 & 45.04 & 7.26 & 15.80 \\ \hline
% %   Median & 7.42 & 5.50 & 7.44 & 18.75 & 9.01 & 12.10 & 61.08 & 14.52 & 34.69 \\ \hline
% %   Mean & 14.40 & 7.42 & 11.56 & 38.06 & 12.86 & 22.69 & 107.71 & 22.48 & 46.85 \\ \hline
% %   3rd \mbox{Quartile} & 12.71 & 8.55 & 10.92 & 32.01 & 14.48 & 25.57 & 103.92 & 27.50 & 63.55 \\ \hline
% %   Maximum & 931.17 & 190.71 & 302.12 & 931.17 & 190.71 & 302.12 & 931.17 & 190.71 & 302.12 \\ \hline
% %   Standard \mbox{Deviation} & 41.77 & 9.04 & 16.71 & 75.23 & 14.80 & 27.32 & 138.94 & 25.82 & 42.31 \\ \hline
% % \end{tabular}
% % \caption{\label{tab: supp-summary} Summary statistics of the monitor observations, Di estimates, and Reid estimates in the smoke validation set (including monitor observations where either the Di or Reid estimate was missing), subset by level of PM$_{2.5}$. All values are in $\mu g/m^3$.}
% % \end{table}

% % \begin{table}[!hb]
% % \centering
% % \begin{tabular}{|p{2cm} | p{1cm} p{1.3cm} |  p{1cm} p{1.3cm} | p{1cm} p{1.3cm}|}
% %   \hline
% %   & \multicolumn{2}{c|}{\textbf{Overall (N = 29,109)}}  & \multicolumn{2}{c|}{\textbf{Medium (N = 7,868)}} & \multicolumn{2}{c|}{\textbf{High (N = 1,737)}} \\
% %   \hline
% % \textbf{Metric} & Di vs. \mbox{Monitor} & Reid vs. \mbox{Monitor} & Di vs. \mbox{Monitor} & Reid vs. \mbox{Monitor} & Di vs. \mbox{Monitor} & Reid vs. \mbox{Monitor} \\ 
% %   \hline
% %   Mean Bias & -6.60 & -2.84 & -23.79 & -15.34 & -80.69 & -60.93 \\ \hline
% %   Normalized Mean Bias & -0.42 & -0.20 & -0.58 & -0.40 & -0.67 & -0.56 \\ \hline
% %   Median \mbox{Absolute} Difference & 3.00 & 2.90 & 10.87 & 8.98 & 43.34 & 34.51 \\ \hline
% %   Median \mbox{Ratio} & 0.77 & 1.06 & 0.44 & 0.65 & 0.22 & 0.49 \\ \hline
% %   Mean \mbox{Ratio} & 1.87 & 2.56 & 0.52 & 0.82 & 0.33 & 0.63 \\ \hline
% %   RMSD & 36.75 & 37.51 & 70.38 & 71.37 & 148.22 & 149.24 \\ \hline
% %   $R^2$ & 0.11 & 0.20 & 0.06 & 0.14 & 0.01 & 0.04 \\ \hline
% %   Spatial RMSD & 28.24 & 23.06 & 110.01 & 96.57 & 170.60 & 154.58 \\ \hline
% %   Temporal RMSD & 11.44 & 9.73 & 70.81 & 65.68 & 185.09 & 180.73 \\ \hline
% %   Spatial \mbox{Correlation} & 0.64 & 0.67 & 0.01 & 0.09 & -0.11 & -0.09 \\ \hline
% %   Temporal \mbox{Correlation} & 0.49 & 0.54 & 0.05 & 0.19 & -0.11 & 0.08 \\ \hline
% % \end{tabular}
% % \caption{\label{tab: supp-metrics} Metrics comparing the Di estimates and Reid estimates to the smoke monitor observations (2008-2016; including monitor observations where either the Di or Reid estimate was missing), stratified by PM$_{2.5}$ level. All metrics except for median ratio, mean ratio, $R^2$, and spatial/temporal correlation are in $\mu g/m^3$.}
% % \end{table}

% \begin{table}[!hb]
% \centering
% \begin{tabular}{|p{3cm} | p{1.5cm} p{1.5cm}  p{1.5cm} | p{1.5cm} p{1.5cm} p{1.5cm}|}
%     \hline
%     & \multicolumn{3}{p{4.5cm}|}{\textbf{\mbox{Reid 2017-2018} \mbox{without} CMAQ}} & \multicolumn{3}{p{4.5cm}|}{\textbf{\mbox{Reid 2008-2016} \mbox{without} CMAQ}} \\
%     \hline
%   \textbf{Metric (\mbox{Optimal} Value)} & \textbf{Overall} \mbox{(N =} 9,662) & \textbf{Medium} \mbox{(N =} 3,463) & \textbf{High} \mbox{(N =} 1,101) & \textbf{Overall} \mbox{(N =} 19,850) & \textbf{Medium} \mbox{(N =} 5,432) & \textbf{High} \mbox{(N =} 1,034)  \\
%   \hline
% Mean Bias (0) & 0.26 & -6.12 & -19.66 & -1.01 & -11.90 & -61.87 \\ 
%   \hline
% Normalized \mbox{Mean Bias (0)} & 0.02 & -0.18 & -0.22 & -0.08 & -0.40 & -0.65 \\ 
%   \hline
% \mbox{Median Absolute} \mbox{Difference} (0) & 2.70 & 7.25 & 19.32 & 2.94 & 5.99 & 33.91 \\ 
%   \hline
% \mbox{Median Ratio (1)} & 1.19 & 0.77 & 0.82 & 1.21 & 0.74 & 0.45 \\ 
%   \hline
%  Mean Ratio (1) & 1.95 & 0.84 & 0.83 & 6.81 & 0.79 & 0.49 \\ 
%   \hline
% RMSD (0) & 13.63 & 27.51 & 54.62 & 28.22 & 54.68 & 144.10 \\ 
%   \hline
% $R^2$ (1) & 0.66 & 0.60 & 0.45 & 0.12 & 0.07 & 0.01 \\ 
%   \hline
% \mbox{Spatial RMSD} (0) & 8.20 & 14.37 & 69.30 & 71.51 & 81.48 & 148.85 \\ 
%   \hline
% \mbox{Temporal RMSD} (0) & 7.47 & 86.85 & 198.85 & 18.60 & 68.14 & 149.01 \\ 
%   \hline
% Spatial \mbox{Correlation (1)} & 0.94 & 0.90 & 0.45 & 0.39 & 0.33 & 0.14 \\ 
%   \hline
% Temporal \mbox{Correlation (1)} & 0.84 & 0.07 & -0.18 & 0.32 & 0.12 & 0.00 \\ 
%   \hline
% \end{tabular}
% \caption{\label{tab: wo-CMAQ compare} Metrics (weighted by population density) comparing the Reid estimates without CMAQ, for both 2017-2018 (Di's estimates only extend till 2016) and 2008-2016 to the smoke monitor (WRCC and Airsys, without missingness) observations, stratified by PM$_{2.5}$ level. All metrics except for median ratio, mean ratio, $R^2$, and spatial/temporal correlation are in $\mu g/m^3$.}
% \end{table}


% \begin{table}[!hb]
% \centering
% \begin{tabular}{|p{3.6cm} | p{1.5cm} p{1.5cm} |  p{1.5cm} p{1.5cm} | p{1.5cm} p{1.5cm}|}
%   \hline
%   & \multicolumn{2}{p{3cm}|}{\textbf{Overall \mbox{(N = 927,414)}}}  & \multicolumn{2}{p{3cm}|}{\textbf{Medium \mbox{(N = 151,935)}}} & \multicolumn{2}{p{3cm}|}{\textbf{High \mbox{(N = 8,707)}}} \\
%   \hline
% \textbf{Metric \mbox{(Optimal Value)}} & Di vs. \mbox{Monitor} & Reid vs. \mbox{Monitor} & Di vs. \mbox{Monitor} & Reid vs. \mbox{Monitor} & Di vs. \mbox{Monitor} & Reid vs. \mbox{Monitor} \\ 
%   \hline
%   Mean Bias (0) & -0.31 & 0.13 & -2.55 & -1.98 & -5.66 & -7.78 \\ 
%   \hline
% Normalized \mbox{Mean Bias (0)} & -0.03 & 0.01 & -0.13 & -0.10 & -0.12 & -0.16 \\ 
%   \hline
% \mbox{Median Absolute} \mbox{Difference} (0) & 1.22 & 1.18 & 2.96 & 2.09 & 7.79 & 6.93 \\ 
%   \hline
% \mbox{Median Ratio (1)} & 0.99 & 1.05 & 0.88 & 0.91 & 0.91 & 0.86 \\ 
%   \hline
%  Mean Ratio (1) & 1.12 & 1.24 & 0.87 & 0.91 & 0.88 & 0.84 \\ 
%   \hline
% RMSD (0) & 3.87 & 2.84 & 6.74 & 4.68 & 19.08 & 13.18 \\ 
%   \hline
% $R^2$ (1) & 0.72 & 0.85 & 0.59 & 0.76 & 0.28 & 0.56 \\ 
%   \hline
% \mbox{Spatial RMSD (0)} & 1.63 & 1.09 & 3.54 & 2.92 & 15.85 & 13.29 \\ 
%   \hline
% \mbox{Temporal RMSD (0)} & 0.82 & 0.67 & 4.21 & 2.76 & 28.74 & 25.40 \\ 
%   \hline
% Spatial \mbox{Correlation (1)} & 0.87 & 0.94 & 0.68 & 0.83 & 0.32 & 0.55 \\ 
%   \hline
% Temporal \mbox{Correlation (1)} & 0.97 & 0.98 & 0.82 & 0.88 & 0.16 & 0.40 \\ 
%   \hline
% \end{tabular}
% \caption{\label{tab: EPA compare} Metrics (weighted by population density) comparing the Di estimates and Reid estimates to the EPA monitor observations from 2008-2016 (on which both models were trained), stratified by PM$_{2.5}$ level. All metrics except for median ratio, mean ratio, $R^2$, and spatial/temporal correlation are in $\mu g/m^3$. Note: the overall $R^2$ values are different from those stated in each model's corresponding paper because (a) the Di model was not evaluated over the entire western US and the predictions were capped at 200 $\mu g/m^3$, and (b) the Reid model was trained and evaluated on a larger dataset than just the EPA monitor data. }
% \end{table}

% \end{document}
