# Supplementary material for: Evaluation of Model-Based PM$_{2.5}$ Estimates for Exposure Assessment During Wildfire Smoke Episodes in the Western U.S
Source: arXiv:2209.01479 source file (2023-01-09)
Supplement: Supplementary file 2 [file Supporting_Information.pdf]

# Supporting Information for "Evaluation of Model-Based PM<sub>2.5</sub> Estimates for Exposure Assessment During Wildfire Smoke Episodes in the Western U.S."

Ellen M. Considine,<sup>\*,†</sup> Jiayuan Hao,<sup>†</sup> Priyanka deSouza,<sup>‡,¶</sup> Danielle Braun,<sup>†,§</sup>

Colleen E. Reid,<sup>||,¶,⊥</sup> and Rachel C. Nethery<sup>†</sup>

<sup>†</sup>*Department of Biostatistics, Harvard T.H. Chan School of Public Health*

<sup>‡</sup>*Department of Urban and Regional Planning, University of Colorado Denver*

<sup>¶</sup>*CU Population Center, University of Colorado Boulder*

<sup>§</sup>*Department of Data Science, Dana-Farber Cancer Institute*

<sup>||</sup>*Department of Geography, University of Colorado Boulder*

<sup>⊥</sup>*Earth Lab, University of Colorado Boulder*

E-mail: ellen\_considine@g.harvard.edu

## Comparison Metrics Equations

$$\text{Mean Bias}(\mathbf{x}, \mathbf{y}) = \frac{1}{n} \sum_{i=1}^n (y_i - x_i) \quad (1)$$

$$\text{Normalized Mean Bias}(\mathbf{x}, \mathbf{y}) = \frac{\sum_{i=1}^n (y_i - x_i)}{\sum_{i=1}^n x_i} \quad (2)$$

$$\text{Median Absolute Difference}(\mathbf{x}, \mathbf{y}) = \text{Median}\left\{|y_i - x_i|\right\}_{i=1}^n \quad (3)$$

$$\text{Median Ratio}(\mathbf{x}, \mathbf{y}) = \text{Median}\left\{y_i/x_i\right\}_{i=1}^n \quad (4)$$

$$\text{Mean Ratio}(\mathbf{x}, \mathbf{y}) = \frac{1}{n} \sum_{i=1}^n (y_i/x_i) I(x_i > 0) \quad (5)$$

$$\text{Root-Mean Squared Difference}(\mathbf{x}, \mathbf{y}) = \sqrt{\frac{1}{n} \sum_{i=1}^n (y_i - x_i)^2} \quad (6)$$

$$R^2(\mathbf{x}, \mathbf{y}) = \left[ \frac{\sum_{i=1}^n (y_i - \bar{y})(x_i - \bar{x})}{\sqrt{\sum_{i=1}^n (y_i - \bar{y})^2 \sum_{i=1}^n (x_i - \bar{x})^2}} \right]^2 \quad (7)$$

For spatial RMSD and  $R^2$ , replace individual observations with location-averages (across all the days). For temporal RMSD and  $R^2$ , replace individual observations with daily averages (across all locations).

## Supplemental Notes

In the Results, we noted that the mean ratio between the Reid estimates and the smoke monitor observations was affected by 25 instances where the monitor observations were in their lowest quartile ( $< 4\mu g/m^3$ ) and the model estimates were high ( $> 35.5\mu g/m^3$ ). Of these, eight of the Reid estimates were over  $55.5 \mu g/m^3$ ; the maximum was  $103.7 \mu g/m^3$ . Among these 25 instances, all but one were in the warm season (and the one was in April). A large cluster of the over-predictions were in northern California in 2015, at a location bordered by half a dozen large fires in its bordering counties. By contrast, the highest three over-predictions were in Colorado in October 2016, at a location sandwiched between two major fires that were each about 150 miles away. Investigating this issue revealed that these

predictions were heavily influenced by one observation in the Reid training data where a monitor reported a concentration of  $781.5 \mu\text{g}/\text{m}^3$ . (It is unclear whether this may have been a sensor error, but the existence of a smoke monitor in the area indicates there was concern about fire smoke.)

## Supplemental Figures and Tables

Table S1: Mean (standard deviation) for each data source and subset in the validation set, by state. All values are in  $\mu\text{g}/\text{m}^3$ .

|                                                                          | <b>Overall (N = 26,770)</b> |                 |                  | <b>Medium (N = 7,216)</b> |                  |                  | <b>High (N = 1,552)</b> |                  |                  |
|--------------------------------------------------------------------------|-----------------------------|-----------------|------------------|---------------------------|------------------|------------------|-------------------------|------------------|------------------|
| <b>Subset<br/>(<math>N_O</math>, <math>N_M</math>, <math>N_H</math>)</b> | MonitorDi                   |                 | Reid             | MonitorDi                 |                  | Reid             | MonitorDi               |                  | Reid             |
| Arizona<br>(180, 13, 1)                                                  | 7.24<br>(5.87)              | 6.3<br>(2.53)   | 6.68<br>(7.15)   | 21.22<br>(14.26)          | 7.53<br>(1.35)   | 21.6<br>(17.14)  | 66.12<br>(NA)           | 8.74<br>(NA)     | 45.79<br>(NA)    |
| California<br>(17925, 5558, 904)                                         | 13.54<br>(23.53)            | 7.53<br>(8.62)  | 12.31<br>(15.91) | 28.43<br>(38.06)          | 11.93<br>(13.5)  | 21.17<br>(24.97) | 82.02<br>(72.96)        | 23.27<br>(26.6)  | 50.27<br>(40.39) |
| Colorado<br>(1353, 136, 80)                                              | 13.16<br>(77.88)            | 3.12<br>(2.92)  | 4.86<br>(11.91)  | 114.5<br>(221.77)         | 5.92<br>(4.64)   | 19.77<br>(27.4)  | 180.15<br>(270.97)      | 6.64<br>(4.32)   | 24.28<br>(30.54) |
| Idaho<br>(2575, 697, 247)                                                | 14.8<br>(33.48)             | 9.62<br>(12.01) | 12.66<br>(16.09) | 42.02<br>(55.68)          | 18.1<br>(19.03)  | 25.32<br>(23.87) | 81.07<br>(79.52)        | 26.28<br>(25.15) | 37.76<br>(26.89) |
| Montana<br>(1332, 223, 64)                                               | 10.47<br>(26.58)            | 8.08<br>(11.95) | 6.87<br>(11.24)  | 42.1<br>(54.58)           | 18.96<br>(24.36) | 19.43<br>(21.26) | 100.64<br>(74.38)       | 38.09<br>(36.88) | 37.71<br>(28.38) |
| New Mexico<br>(1066, 94, 46)                                             | 10.93<br>(50.69)            | 4.98<br>(3.8)   | 8.07<br>(9.49)   | 92.05<br>(148.56)         | 8.8<br>(6.31)    | 20.89<br>(18.36) | 166.23<br>(185.85)      | 6.43<br>(6.21)   | 18.9<br>(19.07)  |
| Oregon<br>(866, 173, 86)                                                 | 20.01<br>(87.76)            | 7.21<br>(7.33)  | 11.09<br>(19.1)  | 89.01<br>(180.89)         | 14.23<br>(11.92) | 31.53<br>(34.7)  | 158.5<br>(237.6)        | 14.58<br>(14.43) | 43.06<br>(43.75) |
| Utah (66, 17, 14)                                                        | 31.14<br>(58.2)             | 2.89<br>(0.9)   | 14.2<br>(16.61)  | 114.81<br>(61.06)         | 2.75<br>(0.6)    | 35.54<br>(20.88) | 134.06<br>(48.18)       | 2.66<br>(0.47)   | 40.51<br>(19.23) |
| Washington<br>(1288, 270, 89)                                            | 20.6<br>(85.47)             | 8.1<br>(11.46)  | 11.4<br>(22.59)  | 80.56<br>(174.2)          | 18.41<br>(19.63) | 28.47<br>(43.43) | 206.01<br>(262.58)      | 28.72<br>(27.72) | 57.05<br>(65.32) |
| Wyoming<br>(119, 35, 21)                                                 | 35.17<br>(94.53)            | 7.2<br>(6.94)   | 13.44<br>(16.21) | 112.75<br>(149.06)        | 14.44<br>(8.65)  | 32.52<br>(16.85) | 173.26<br>(167.72)      | 15.27<br>(10.49) | 35.89<br>(15.71) |

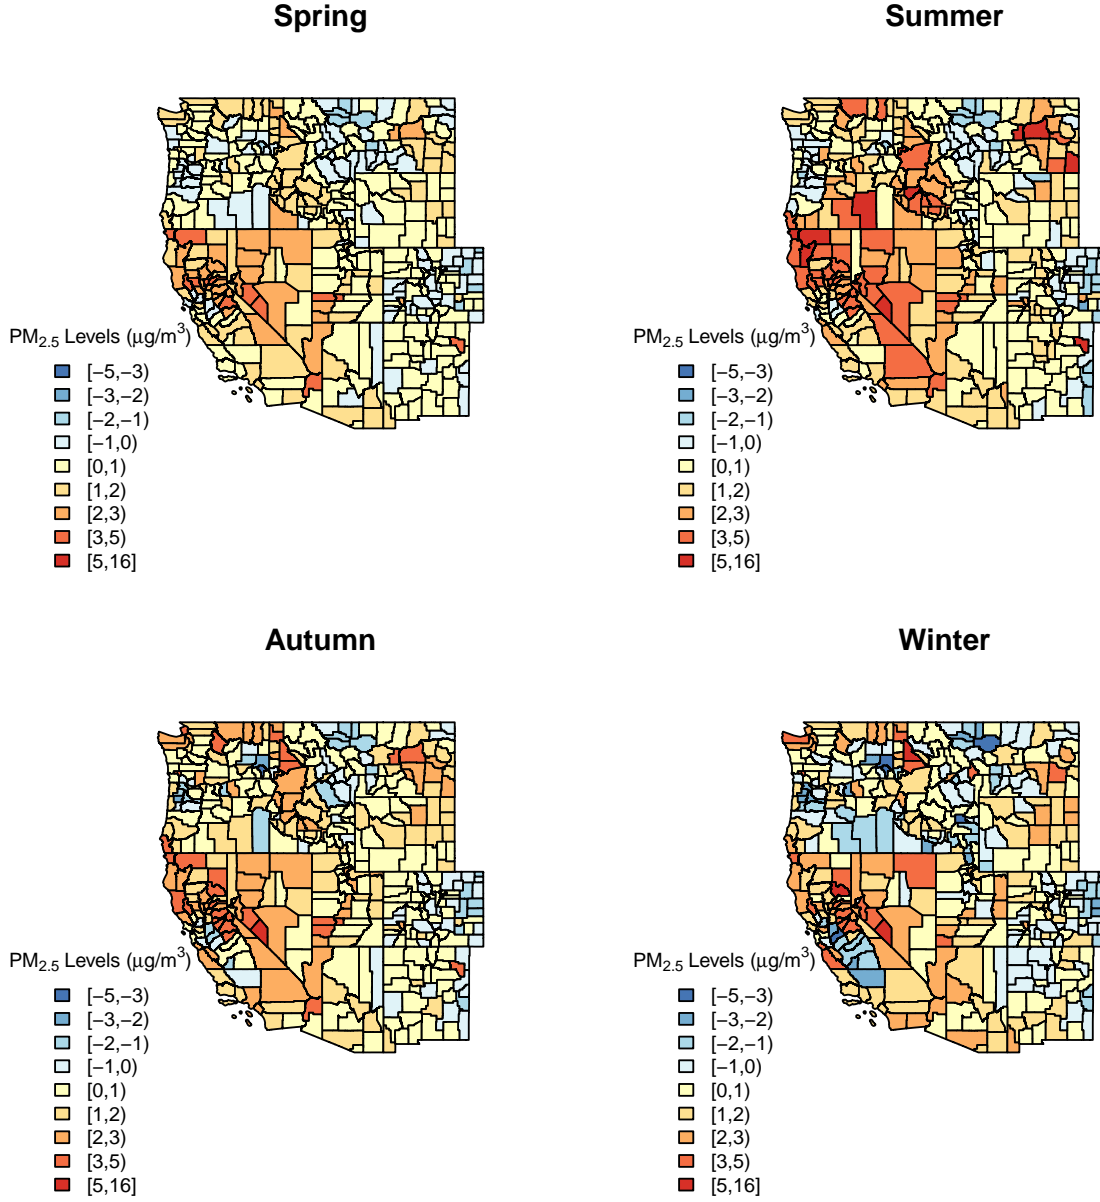

Figure S1: Maps of the seasonal differences (Reid - Di) between county-level averages (2008-2016) of the model-based estimates. We define Spring as March-May, Summer as June-August, Autumn as September-November, and Winter as December-February.

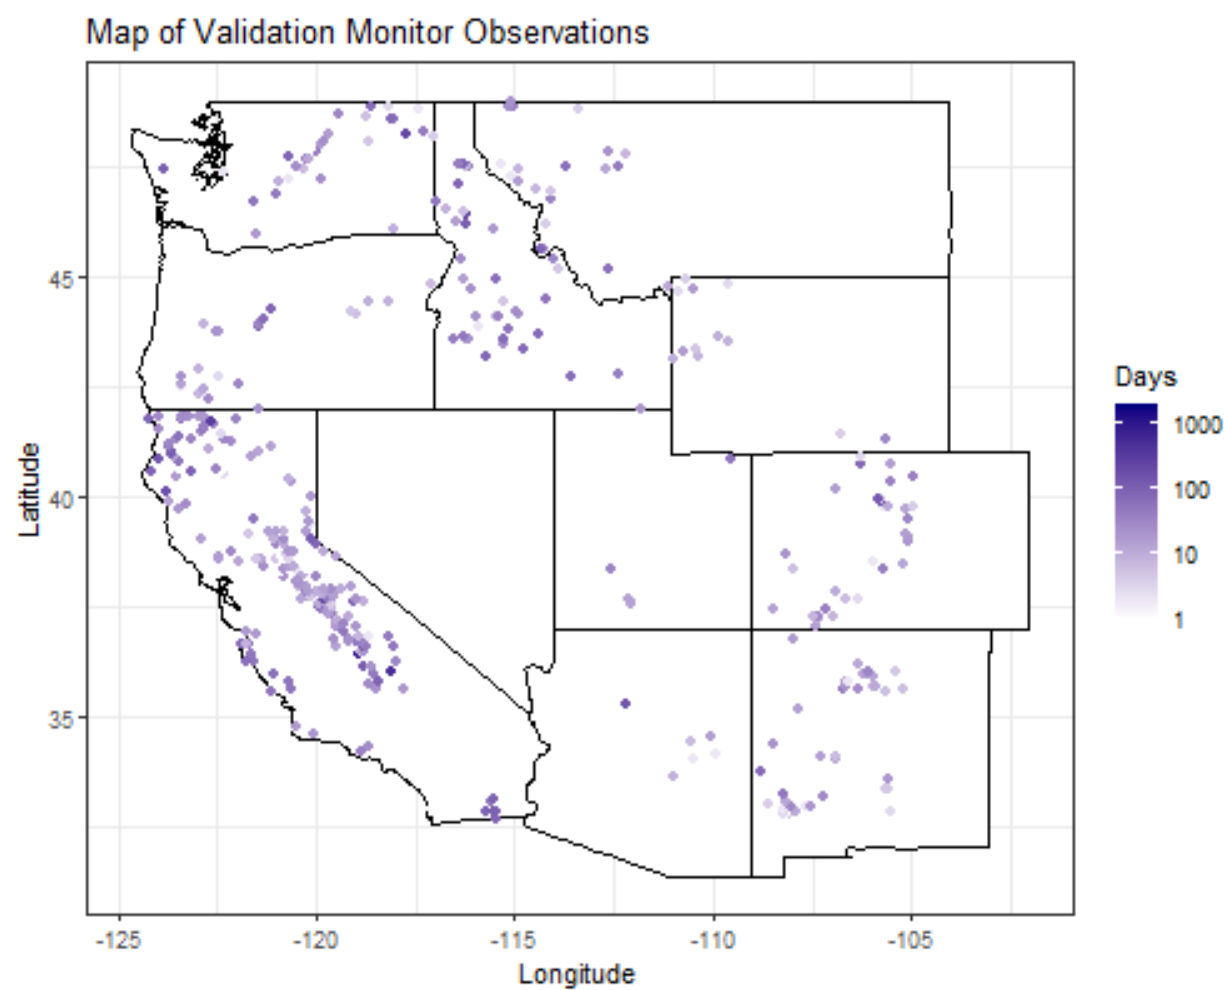

Figure S2: Map of all smoke monitor observations in the validation set, colored by the number of days they were deployed.

Table S2: Frequency tables for the Di and Reid estimates' classification of the AQI in the validation set. Levels 1-6 of the AQI are described in Methods: Analysis.

|                    | Di AQI Class |      |     |     |     |      |           |
|--------------------|--------------|------|-----|-----|-----|------|-----------|
| Monitor AQI Class  | 1            | 2    | 3   | 4   | 5   | 6    | Marginals |
| 1                  | 18667        | 851  | 13  | 9   | 0   | 0    | 19540     |
| 2                  | 4144         | 1421 | 67  | 24  | 0   | 0    | 5656      |
| 3                  | 311          | 301  | 42  | 29  | 0   | 0    | 683       |
| 4                  | 262          | 263  | 73  | 44  | 6   | 0    | 648       |
| 5                  | 40           | 40   | 10  | 24  | 1   | 0    | 115       |
| 6                  | 53           | 20   | 6   | 21  | 4   | 0    | 104       |
| Marginals          | 23477        | 2896 | 211 | 151 | 11  | 0    | 26746     |
| Percent Change (%) | +20          | -49  | -69 | -77 | -90 | -100 |           |

(a) Di classifications compared to smoke monitor classifications

|                    | Reid AQI Class |      |     |     |     |     |           |
|--------------------|----------------|------|-----|-----|-----|-----|-----------|
| Monitor AQI Class  | 1              | 2    | 3   | 4   | 5   | 6   | Marginals |
| 1                  | 17603          | 1769 | 116 | 52  | 0   | 0   | 19540     |
| 2                  | 3348           | 1824 | 295 | 187 | 2   | 0   | 5656      |
| 3                  | 157            | 269  | 127 | 128 | 2   | 0   | 683       |
| 4                  | 101            | 201  | 134 | 201 | 11  | 0   | 648       |
| 5                  | 16             | 12   | 13  | 63  | 11  | 0   | 115       |
| 6                  | 34             | 8    | 9   | 40  | 11  | 2   | 104       |
| Marginals          | 21259          | 4083 | 694 | 671 | 37  | 2   | 26746     |
| Percent Change (%) | +9             | -28  | +2  | +4  | -68 | -98 |           |

(b) Reid classifications compared to smoke monitor classifications

Table S3: AQI classification metrics for the Di and Reid estimates compared with the smoke monitor observations.

| Comparison      | Misclassified | Underclassified | Overclassified | Large Misclass. |
|-----------------|---------------|-----------------|----------------|-----------------|
| Di vs Monitor   | 24.57         | 20.83           | 3.74           | 4.01 %          |
| Reid vs Monitor | 26.09         | 16.51           | 9.58           | 3.55 %          |

Table S4: Frequency tables for the Di and Reid estimates' binary classification of AQI as Non-smoke ("Good" or "Moderate") vs. Smoke ("Unhealthy for Sensitive Groups" and above) in the validation set.

|                         | Di Binary Exposure |       |           |
|-------------------------|--------------------|-------|-----------|
| Monitor Binary Exposure | Non-smoke          | Smoke | Marginals |
| Non-smoke               | 25083              | 113   | 25196     |
| Smoke                   | 1290               | 260   | 1550      |
| Marginals               | 26373              | 373   | 26746     |

(a) Di classifications compared to smoke monitor classifications

|                         | Reid Binary Exposure |       |           |
|-------------------------|----------------------|-------|-----------|
| Monitor Binary Exposure | Non-smoke            | Smoke | Marginals |
| Non-smoke               | 24544                | 652   | 25196     |
| Smoke                   | 798                  | 752   | 1550      |
| Marginals               | 25342                | 1404  | 26746     |

(b) Reid classifications compared to smoke monitor classifications

Table S5: Summary statistics for the Di and Reid estimates' binary classification of AQI as Non-smoke ("Good" or "Moderate") vs. Smoke ("Unhealthy for Sensitive Groups" and above) in the smoke monitor validation set. PPV = positive predictive value, NPV = negative predictive value.

| Comparison      | Misclassified | Sensitivity | Specificity | PPV     | NPV     |
|-----------------|---------------|-------------|-------------|---------|---------|
| Di vs Monitor   | 5.25 %        | 16.77 %     | 99.55 %     | 69.71 % | 95.11 % |
| Reid vs Monitor | 5.42%         | 48.52 %     | 97.41 %     | 53.56 % | 96.85 % |

Table S6: Summary statistics of the monitor observations, Di estimates, and Reid estimates in the smoke validation set (including monitor observations where either the Di or Reid estimate was missing), subset by level of PM<sub>2.5</sub>. All values are in  $\mu\text{g}/\text{m}^3$ .

|                    | Overall (N = 29,109) |        |        | Medium (N = 7,868) |        |        | High (N = 1,737) |        |        |
|--------------------|----------------------|--------|--------|--------------------|--------|--------|------------------|--------|--------|
| Metric             | Monitor              | Di     | Reid   | Monitor            | Di     | Reid   | Monitor          | Di     | Reid   |
| Minimum            | 0.00                 | 0.00   | 0.00   | 12.12              | 0.00   | 0.14   | 35.50            | 0.00   | 0.63   |
| 1st Quartile       | 4.04                 | 3.32   | 4.80   | 14.50              | 5.75   | 8.10   | 45.04            | 7.26   | 15.80  |
| Median             | 7.42                 | 5.50   | 7.44   | 18.75              | 9.01   | 12.10  | 61.08            | 14.52  | 34.69  |
| Mean               | 14.40                | 7.42   | 11.56  | 38.06              | 12.86  | 22.69  | 107.71           | 22.48  | 46.85  |
| 3rd Quartile       | 12.71                | 8.55   | 10.92  | 32.01              | 14.48  | 25.57  | 103.92           | 27.50  | 63.55  |
| Maximum            | 931.17               | 190.71 | 302.12 | 931.17             | 190.71 | 302.12 | 931.17           | 190.71 | 302.12 |
| Standard Deviation | 41.77                | 9.04   | 16.71  | 75.23              | 14.80  | 27.32  | 138.94           | 25.82  | 42.31  |

Table S7: Metrics comparing the Di estimates and Reid estimates to the smoke monitor observations (2008-2016; including monitor observations where either the Di or Reid estimate was missing), stratified by PM<sub>2.5</sub> level. All metrics except for median ratio, mean ratio,  $R^2$ , and spatial/temporal correlation are in  $\mu g/m^3$ .

|                                  | <b>Overall (N = 29,109)</b> |                        | <b>Medium (N = 7,868)</b> |                        | <b>High (N = 1,737)</b> |                        |
|----------------------------------|-----------------------------|------------------------|---------------------------|------------------------|-------------------------|------------------------|
| <b>Metric</b>                    | Di<br>vs.<br>Monitor        | Reid<br>vs.<br>Monitor | Di<br>vs.<br>Monitor      | Reid<br>vs.<br>Monitor | Di<br>vs.<br>Monitor    | Reid<br>vs.<br>Monitor |
| Mean Bias                        | -6.60                       | -2.84                  | -<br>23.79                | -15.34                 | -<br>80.69              | -60.93                 |
| Normalized<br>Mean Bias          | -0.42                       | -0.20                  | -0.58                     | -0.40                  | -0.67                   | -0.56                  |
| Median<br>Absolute<br>Difference | 3.00                        | 2.90                   | 10.87                     | 8.98                   | 43.34                   | 34.51                  |
| Median<br>Ratio                  | 0.77                        | 1.06                   | 0.44                      | 0.65                   | 0.22                    | 0.49                   |
| Mean<br>Ratio                    | 1.87                        | 2.56                   | 0.52                      | 0.82                   | 0.33                    | 0.63                   |
| RMSD                             | 36.75                       | 37.51                  | 70.38                     | 71.37                  | 148.22                  | 149.24                 |
| $R^2$                            | 0.11                        | 0.20                   | 0.06                      | 0.14                   | 0.01                    | 0.04                   |
| Spatial<br>RMSD                  | 28.24                       | 23.06                  | 110.01                    | 96.57                  | 170.60                  | 154.58                 |
| Temporal<br>RMSD                 | 11.44                       | 9.73                   | 70.81                     | 65.68                  | 185.09                  | 180.73                 |
| Spatial<br>Correlation           | 0.64                        | 0.67                   | 0.01                      | 0.09                   | -0.11                   | -0.09                  |
| Temporal<br>Correlation          | 0.49                        | 0.54                   | 0.05                      | 0.19                   | -0.11                   | 0.08                   |

Table S8: Metrics comparing the Reid estimates without CMAQ, for both 2017-2018 (Di's estimates only extend till 2016) and 2008-2016 to the smoke monitor (WRCC and Airsys, without missingness) observations, stratified by PM<sub>2.5</sub> level. All metrics except for median ratio, mean ratio,  $R^2$ , and spatial/temporal correlation are in  $\mu g/m^3$ .

|                            | <b>Reid 2017-2018 without CMAQ</b> |                              |                            | <b>Reid 2008-2016 without CMAQ</b> |                              |                            |
|----------------------------|------------------------------------|------------------------------|----------------------------|------------------------------------|------------------------------|----------------------------|
| <b>Metric</b>              | <b>Overall</b><br>(N = 14,316)     | <b>Medium</b><br>(N = 5,068) | <b>High</b><br>(N = 1,793) | <b>Overall</b><br>(N = 26,863)     | <b>Medium</b><br>(N = 7,246) | <b>High</b><br>(N = 1,575) |
| Mean Bias                  | -1.01                              | -10.08                       | -33.70                     | -2.08                              | -15.40                       | -60.55                     |
| Normalized Mean Bias       | -0.05                              | -0.20                        | -0.31                      | -0.15                              | -0.42                        | -0.59                      |
| Median Absolute Difference | 4.22                               | 9.93                         | 28.73                      | 3.56                               | 8.77                         | 36.05                      |
| Median Ratio               | 1.28                               | 0.87                         | 0.75                       | 1.17                               | 0.65                         | 0.42                       |
| Mean Ratio                 | 2.42                               | 1.05                         | 0.87                       | 4.61                               | 0.80                         | 0.58                       |
| RMSD                       | 41.42                              | 68.68                        | 112.68                     | 36.05                              | 68.50                        | 145.22                     |
| $R^2$                      | 0.40                               | 0.31                         | 0.16                       | 0.18                               | 0.13                         | 0.05                       |
| Spatial RMSD               | 38.24                              | 54.53                        | 85.66                      | 24.03                              | 93.91                        | 154.56                     |
| Temporal RMSD              | 13.08                              | 89.05                        | 183.93                     | 10.43                              | 67.87                        | 173.94                     |
| Spatial Correlation        | 0.78                               | 0.64                         | 0.34                       | 0.65                               | 0.14                         | 0.00                       |
| Temporal Correlation       | 0.77                               | 0.09                         | -0.12                      | 0.47                               | 0.23                         | 0.15                       |

Table S9: Metrics comparing the Di estimates and Reid estimates to the EPA monitor observations from 2008-2016 (on which both models were trained), stratified by  $\text{PM}_{2.5}$  level. All metrics except for median ratio, mean ratio,  $R^2$ , and spatial/temporal correlation are in  $\mu\text{g}/\text{m}^3$ . Note: the overall  $R^2$  values are different from those stated in each model’s corresponding paper because (a) the Di model was not evaluated over the entire western US and the predictions were capped at  $200 \mu\text{g}/\text{m}^3$ , and (b) the Reid model was trained and evaluated on a larger dataset than just the EPA monitor data.

|                                  | <b>Overall (N = 928,883)</b> |                        | <b>Medium (N = 151,957)</b> |                        | <b>High (N = 8,710)</b> |                        |
|----------------------------------|------------------------------|------------------------|-----------------------------|------------------------|-------------------------|------------------------|
| <b>Metric</b>                    | Di<br>vs.<br>Monitor         | Reid<br>vs.<br>Monitor | Di<br>vs.<br>Monitor        | Reid<br>vs.<br>Monitor | Di<br>vs.<br>Monitor    | Reid<br>vs.<br>Monitor |
| Mean Bias                        | -0.29                        | -0.08                  | -3.23                       | -3.84                  | -9.85                   | -13.02                 |
| Normalized<br>Mean Bias          | -0.04                        | -0.01                  | -0.16                       | -0.20                  | -0.20                   | -0.26                  |
| Median<br>Absolute<br>Difference | 1.18                         | 1.34                   | 3.49                        | 2.99                   | 10.22                   | 9.82                   |
| Median<br>Ratio                  | 0.99                         | 1.06                   | 0.85                        | 0.86                   | 0.85                    | 0.82                   |
| Mean<br>Ratio                    | 1.19                         | 1.45                   | 0.85                        | 0.82                   | 0.81                    | 0.75                   |
| RMSD                             | 4.25                         | 4.38                   | 8.73                        | 9.07                   | 25.66                   | 25.45                  |
| $R^2$                            | 0.67                         | 0.64                   | 0.49                        | 0.46                   | 0.20                    | 0.25                   |
| Spatial<br>RMSD                  | 1.48                         | 1.76                   | 5.46                        | 6.07                   | 21.26                   | 20.66                  |
| Temporal<br>RMSD                 | 0.70                         | 0.88                   | 4.63                        | 4.48                   | 28.53                   | 27.17                  |
| Spatial<br>Correlation           | 0.90                         | 0.85                   | 0.56                        | 0.54                   | 0.27                    | 0.40                   |
| Temporal<br>Correlation          | 0.97                         | 0.95                   | 0.83                        | 0.81                   | 0.21                    | 0.41                   |
